# Supplementary material for: Learning Optimal Contracts: How to Exploit Small Action Spaces
Source: arXiv:2309.09801 source file (2024-06-07)
Supplement: Supplementary file 1 [file appendix_proofs.tex]

\section{Omitted Proofs}
%\empiricaldist*
\begin{proof}
Let $\widetilde{F} \in \Delta_\Omega$ be the empirical mean distribution returned by Algorithm~\ref{alg:action_oracle} with $q$ \emph{i.i.d} samples drawn according to $F \in \Delta_\Omega$, where each $\omega \in \Omega$
has probability $F_\omega$ of being sampled. Therefore, $\widetilde{F}$ is a random vector supported on $\Delta_\Omega$ 
with expectation $\mathbb{E}[\widetilde{F}_\omega]=F_\omega$ for each $\omega \in \Omega$. Moreover, by Hoeffding’s inequality we have that, for each $\omega \in \Omega$,
\begin{equation}\label{eq:hoeffding}
\mathbb{P}\left(|\widetilde{F}_\omega-\mathbb{E}\left[\widetilde{F}_\omega\right]| \ge \epsilon\right) =\mathbb{P}\left(|\widetilde{F}_\omega-F_\omega| \ge \epsilon\right) \ge 1- 2e^{-q\epsilon^2}.
\end{equation}
Then, by employing union bound and Equation \ref{eq:hoeffding} we have that:
\begin{equation*}
\mathbb{P}\left( \|F-\widetilde{F}\|_{\infty} \le \epsilon \right) = \mathbb{P}\left(\bigcap_{\omega \in \Omega }\{ |F_\omega-\widetilde{F}_\omega| \le \epsilon \}\right) \ge 1 - 2 m e^{-q\epsilon^2} \ge 1-\alpha.
\end{equation*}
where the last inequality holds because of the definition of $q$.
\end{proof}

%\boundedactions*
\begin{proof} 

In the following we let $F_{i,j} \in \mathcal{F}_{a_{i^*}}$ be the empirical distribution (observed by the principal) such that $\|F_{i,j} - F_{i}\|_{\infty} \le 2\epsilon$ and $\|F_{i,j} - F_{j}\|_{\infty} \le 2\epsilon$, with $F_i \in B_\epsilon(F_{a_i})$ and $F_{j} \in B_\epsilon(F_{a_{j}})$, where we denote $B_\epsilon(F) \coloneqq \{F' \in \Delta_\Omega \, | \, \| F - F' \|_{\infty} \le \epsilon   \}$. By Lemma~\ref{lem:hoeffding} we know that $F_i \in B_\epsilon(F_{a_i})$ and $F_{j} \in B_\epsilon(F_{a_{j}})$ with sufficiently high probability.

\alb{Sopra non si capisce cosa sono quelle distribuzioni.}

We observe that, for each couple of actions $a_{i_1}, a_{i_2} \in \mathcal{A}$ with $i_1,i_2 \in I$ there exists a $I'=\{i_1, \dots, i_2\} \subseteq I$ and a sequence of empirical distributions $\{ F_{i,i+1}\}_{i \in I'} \subseteq \mathcal{F}_{a_i^*}$ define as above. This is because \ActionOracle identifies action $a_{i_1}$ and action $ a_{i_2}$ as a single one. We first we observe that for each $i \in I'$ it holds:
\begin{align*}
\| F_{a_{i}} - F_{a_{i+1}}\|_{\infty} & =   \| F_{a_{i}} - F_{i} + F_{i} - F_{i,i+1} + F_{i,i+1}  - F_{i+1} + F_{i+1} - F_{a_{i+1}}\|_{\infty} \\
& =   \| F_{a_{i}} - F_{i}  \|_{\infty} + \| F_{i} - F_{i,i+1}  \|_{\infty} +  \| F_{i,i+1} - F_{i+1}\|_{\infty} + \| F_{i+1} - F_{a_{i+1}} \|_{\infty} \\
& \le 5 \epsilon.
\end{align*}
Then we have:
\begin{equation*}
 \| F_{a_{i_1}} - F_{a_{i_2}} \|_{\infty} = \| \sum_{i \in I'} F_{a_{i}} - F_{a_{i+1}} \|_{\infty} \le \sum_{i \in I'} \| F_{a_{i}} - F_{a_{i+1}}\|_{\infty} \le 5 \epsilon |I'| \le 5 \epsilon n.
\end{equation*}
Since the latter argument holds for each pair of $i_1,i_2 \in I$, the proof is concluded.
\end{proof}

%\complexity*
\begin{proof}
	%First we observe that the algorithm terminates in a finite number of steps. This is because at each iteration of the while-loop at lines we either discover a new hyperplane or the algorithm exit the while-loop. Such an hyperplane is new since $p \in \mathcal{U}_{d}$ and $d \in \mathcal{D}$ is not implemented in $\mathcal{P}_{a}$. Furthermore we observe that during the interaction we never encounter the same hyperplane more then once. This is because when we discover an hyperplane we update the lowerbound of the two regions it separrating.
	
	To derive the sample complexity of the algorithm we first observe that the number of vertices of the regions $\mathcal{U}_{d}$ for each $d \in \mathcal{D}$ is bounded by $\binom{h(\preg) + n}{m} $. This is because the hyperplanes defining the regions $\mathcal{U}_{d}$ are a subset of the $n$ hyperplanes separating a feasibility region from the other ones and the $h(\mathcal{P})$ hyperplanes defining the boundaries of the region $\mathcal{P}$. Consequently, since each vertex lies at most at the intersection of $m$ linear independent hyperplanes we have that the total number of vertexes of the regions $\mathcal{U}_{a_i}$ is bounded by $\binom{h(\preg)+ n}{m} $. Consequently, the while-loop at lines ... enumerates among the vertices of the regions $\mathcal{U}_d$ and thus requires at most $\binom{h(\preg)+ n}{m} q $ samples where we let $q$ the number of smaples required by \ActionOracle. During the execution of the while-loop al lines we may identify a separating hyperplane. The sumber of samples required by \texttt{FIND-SEPARATE-HYPERPLANE}i s of at most $\mathcal{O} \log \left(  \frac{1}{\eta}\right) q $. As a further observation we notice that the while-loop at lines may be invoked at most $n$ times, whch the number of hyperplanes bounding the feasibility regions.
\end{proof}

%\epslowerbounds*
\begin{proof}
    In the following we let $I(a_{i^*})$ be the set of action played when \ActionOracle returns $a_{i^*} \in \mathcal{D}$, while we let $I(a_{j^*})$ be the set of action played when \ActionOracle returns $a_{j^*} \in \mathcal{D}$. To prove the lemma we observe that if $p^* \in V(\mathcal{L}_{a})$ then the action $a^* \in \mathcal{D}$ implemented in $p^*$ is $a_{i^*}$ or $a_{j^*}$ as long as $p^* \in H_{i^*j^*}$. We first consider the case in which $\texttt{ACTION-ORACLE}(p^*)$ returns $a_{j^*} \ne a_{i^*}$ with $p^* \in H_{i^*j^*}$. Then the following inequalities hold:
    \begin{align}\label{eq:epsilon_br}
       \sum_{\omega \in \Omega} {F}_{a_i,\omega} p^*_{\omega} - {c}_{a_i} & \ge \sum_{\omega \in \Omega} \widetilde{F}_{a_{i^*},\omega} p^*_{\omega} - {c}_{a_{i}}  - 6 \epsilon m n \\
       & \ge \sum_{\omega \in \Omega} \widetilde{F}_{a_{i^*},\omega}  p^*_{\omega} - {c}_{a_{i}} - (\widetilde{c}_{a_{i^*}} - \widetilde{c}_{a_{j^*}} ) - 6 \epsilon m n - 2\epsilon m, \\
       & = \sum_{\omega \in \Omega} \widetilde{F}_{a_{j^*},\omega}  p^*_{\omega} -  c_{a_i} - 6 \epsilon m  - 2\epsilon m, \\
       & \ge \sum_{\omega \in \Omega} {F}_{a_{j},\omega}  p^*_{\omega}  -  c_{a_i} -14\epsilon m n, 
     \end{align}
where the first equality holds since $p^* \in H_{i^*j^*}$, while the first and the fourth inequality hold because $\| F_{a_i} - \widetilde{F}_{a_{j^*}}\|_{\infty} \le 6 \epsilon n$ for each $a_i \in I(a)$ by Lemma~\ref{lem:boundedactions}. Furthermore we observe that by Carathéodory's theorem we can decompose the contract $p^{*} \in \mathcal{L}_{a}$ as a convex combination of the vertexes of the region $\mathcal{L}_{a}$. Formally :
\begin{equation}\label{eq:pstar}
    \sum_{p^k \in V(\mathcal{L}_{a}) } \alpha(p^{k}) p^{k}_\omega = p^{*}_\omega,
\end{equation}
 for each $\omega \in \Omega$, with $\alpha(p^{k}) \ge 0$ for each $p^{k} \in V(\mathcal{L}_{a}) $ and $\sum_{p^{k} \in V(\mathcal{L}_{a})} \alpha(p^{k}) = 1$. Finally, we notice that for each $p \in V(\mathcal{L}_{a})$ and $a_i \in I(a)$ we have:
\begin{align*}
     \sum_{\omega  \in \Omega }  F_{a(p^*),\omega}  {p}^*_\omega - c_{a(p^*)} & =  \sum_{\omega  \in \Omega } F_{a(p^*),\omega}  \left( \sum_{p^k \in V(\mathcal{L}_{a}) } \alpha(p^k) p^k_\omega \right) - c_{a(p^*)} \\
     & = \sum_{p^k \in V(\mathcal{L}_{a}) } \alpha(p^k) \left( \sum_{\omega  \in \Omega }  F_{a(p^*),\omega} p^{k}_\omega - c_{a(p^*)} \right) \\
     & \le \sum_{p^k \in V(\mathcal{L}_{a}) } \alpha(p^k) \left( \sum_{\omega  \in \Omega }  F_{a_i,\omega} p^{k}_\omega - c_{a_i} + \epsilon' \right)    \\
     & =  \sum_{\omega  \in \Omega }  F_{a_{i},\omega} \left( \sum_{p^k \in V(\mathcal{L}_{a}) } \alpha(p^{k}) p^{k}_\omega \right) - c_{a_{i}} + \epsilon'\\
     & =  \sum_{\omega  \in \Omega }  F_{a_{i},\omega} p^{*}_\omega  - c_{a_{i}} + \epsilon',
 \end{align*}
where the first and the last equality hold because of Equation~\ref{eq:pstar}, while the second and the fourth equality hold because $\sum_{p^{k} \in V(\mathcal{L}_{a})} \alpha(p^{k}) = 1$, while the inequality holds because of Inequality~\ref{eq:epsilon_br} with $\epsilon'= 14 \epsilon n m$, concluding the proof.
\end{proof}

\epsilonsolution*
\begin{proof}
    Let $I(a) \subseteq \mathcal{A}$ be the set of action(s) played by the agent when \ActionOracle returns $a \in \mathcal{D}$. In the following we let $p^* \in \mathcal{P}$ be the contract providing the highest principal's expected utility. To prove the theorem we first consider the case in which $a(p) \in I(a)$ for some $a \in \mathcal{D}$. By Lemma~\ref{lem:boundedactions} we know that $\| F_{a_i} - F_{a_{i'}} \|_{\infty} \le 5\epsilon n $ for each $i,i' \in I(a)$ while, by Lemma~\ref{lem:hoeffding} we have $\| F_{a_i} - F_{a_i}' \|_{\infty} \le \epsilon$, for each empirical distribution $F_{a_i}' \in \Delta_{\Omega}$ observed by the principal when the action played by the agent is equal to $a_i \in \mathcal{A}$. Consequently, for each action $a \in \mathcal{D}$,
    the empirical distribution $F'_{a}$ employed in Algorithm~\ref{alg:separate_search} satisfies:
    \begin{equation}\label{eq:deltadistribution}
        \| F'_{a} - F_{a_{i'}} + F_{a_{i'}} - F_{a_{i}} \|_{\infty} \le \| F'_{a} - F_{a_{i'}}\|_{\infty} + \| F_{a_{i'}} - F_{a_{i}} \|_{\infty} \le  \epsilon + 5 n \epsilon  \le 6 n \epsilon ,
    \end{equation}
    for each $i \in I(a)$, where we let $a_{i'} \in I(a)$ be the action such that $F_a' \in B_{\epsilon}(F_{a_{i'}})$. Furthermore, by means of the latter inequality we notice that in each $p \in \mathcal{P}$ the actual principal's utility and the one estimated by means of $F_{a}' \in \Delta_{\Omega}$ with $a \in \mathcal{D}$ are such that:
    \begin{equation*}
        |  \sum_{\omega  \in \Omega }  (F_{a,\omega} - F_{a,\omega}' )  \left(  r_\omega - {p}_\omega \right) | \le \| F_{a_i} - F_{a}' \|_{\infty} m \le 6 \epsilon n m,
    \end{equation*}
    thanks to Inequality~\ref{eq:deltadistribution} and Holder's inequality. It is important to the remark that to rely on Inequality~\ref{eq:deltadistribution} we must have $a(p) \in I(a)$ for some $a \in \mathcal{D}$, meaning that we have discovered the action $a(p)$ and consequently estimated $F_{a(p)}$ during the execution of the algorithm. 
    
    We switch now the attention to the case in which $a(p^*) \not \in I(a)$ for each $a \in \mathcal{D}$. First we notice that $p^* \in \mathcal{L}_{a}$ for some $a \in \mathcal{D}$, then by Lemma for each $i \in I(a)$ it holds:
    \begin{equation*}
       2 \epsilon m \ge (F_{a(p^*)}-F_{a_{i}}) p^* + c_{a_i}- c_{a(p^*)} \ge 0.
    \end{equation*}
    We now consider the contract $p^{L} \coloneqq (1-\sqrt{\epsilon})p^*  + \sqrt{\epsilon} r$. As a first observation we notice that $p^L \in \mathcal{P}$ since $r \in \mathcal{P}$. Furthermore we notice that either $a(p^L) \in I(a)$ for some $a \in \mathcal{D}$ or there is no $a \in \mathcal{D}$ such that $a(p^L) \in I(a)$. If the first case holds, by means of Lemma~Dutting and the previous analysis, we have that the principal's utility in $p^L \in \mathcal{L}_{a}$ estimated by Algorithm is of at least:
    \begin{align*}
        \sum_{\omega \in \Omega} F_{a(p^*), \omega} \left( r_\omega - p^*_\omega \right)
        & \ge  \sum_{\omega \in \Omega} F_{a(p^L), \omega} \left( r_\omega - p^L_\omega \right)  -\sqrt{ \epsilon m}\\
        & \ge  \sum_{\omega \in \Omega} F'_{a, \omega} \left( r_\omega - p^L_\omega \right)  -\sqrt{ \epsilon m}- 6 \epsilon n m .
    \end{align*}
    We now consider the case in which there is no $a \in \mathcal{D}$ such that $a(p^L) \in I(a)$. In the following we let $a' \in \mathcal{D}$ be the action such that $p^L \in \mathcal{L}_{a'}$, while we let $a \in \mathcal{D}$ be the action such that $p^* \in \mathcal{L}_{a}$. Then for each $a_i \in I(a')$ it holds: 
    \begin{align*}
        \sum_{\omega \in \Omega} F_{a_i, \omega} \left( r_\omega - p^L_\omega \right)
        & =  \sum_{\omega \in \Omega} F_{a_i, \omega} \left( r_\omega - (1-\sqrt{\epsilon}) p_\omega^* + \sqrt{\epsilon} r_\omega ) \right) \\
        & \ge  \sum_{\omega \in \Omega} F_{a_i, \omega} \left( r_\omega - p^*_\omega \right)  -\sqrt{ \epsilon} \sum_{\omega \in \Omega} F_{a_i, \omega} \left( r_\omega - p^*_\omega \right)\\
        & \ge  \sum_{\omega \in \Omega} F_{a_i, \omega} \left( r_\omega - p^*_\omega \right)  -\sqrt{ \epsilon} m,
    \end{align*}
     where the latter inequality holds by observing that $|\sum_{\omega \in \Omega} F_{a_i, \omega} \left( r_\omega - p^*_\omega \right)| \le m $. Furthermore we show that the following inequality holds:\\
     To prove the third statement we observe that if $p' \in co(\bigcup_{i \in I} \mathcal{P}_{a_i})$, then $a_i$ is an $\epsilon$-BR for each $i \in I$ in $p'$. then we have:
     \begin{equation}\label{eq:ineq}
          \epsilon \ge (F_{a_{i^*}} - F_{a_i} ) p^* + c_{a_i}- c_{a_{i^*}} \ge 0,
      \end{equation}
      for each $a_i \in I(a')$
      \begin{align*}
          & \epsilon \ge \sum_{\omega \in \Omega }(F_{a(p^L),\omega} - F_{a_i,\omega} ) p^L_\omega + c_{a_i}- c_{a(p^L)} \\
          & \ge \sum_{\omega \in \Omega }(F_{a(p^*),\omega} - F_{a_i,\omega} ) p^L_\omega + c_{a_i}- c_{a(p^*)} \\
          & = \sum_{\omega \in \Omega }(F_{a(p^*),\omega} - F_{a_i,\omega} ) p^*_\omega  + c_{a_i}- c_{a(p^*)} + \sqrt{\epsilon} \sum_{\omega \in \Omega } (F_{a(p^*),\omega} - F_{a_i,\omega} ) ( r_\omega - p^*_\omega )\\
          & \ge \sqrt{\epsilon} \sum_{\omega \in \Omega } (F_{a(p^*),\omega} - F_{a_i,\omega} ) ( r_\omega - p^*_\omega ),
      \end{align*}
    where in the last step we employed Inequality~\ref{eq:ineq}.
    \begin{equation*}
        \sum_{\omega \in \Omega }F_{a_i,\omega} ( r_\omega - p^*_\omega ) \ge \sum_{\omega \in \Omega }F_{a(p^*),\omega}  ( r_\omega - p^*_\omega )- \sqrt{\epsilon}
    \end{equation*}
\end{proof}
