# Supplementary material for: Learning Optimal Contracts: How to Exploit Small Action Spaces
Source: arXiv:2309.09801 source file (2024-06-07)
Supplement: Supplementary file 2 [file appendix_images.tex]

\section{Related works}\label{sec:related}

In this section, we survey the previous works that are most related to ours.
Among the works addressing principal-agent problems, we only discuss those focusing on learning aspects.
Notice that there are several works studying computational properties of principal-agent problems  which are \emph{not} concerned with learning aspects, such as, \emph{e.g.},~\citep{dutting2019simple,alon2021contracts,guruganesh2021contracts,dutting2021complexity,dutting2022combinatorial,castiglioni2022bayesian,castiglioni2022designing}.

\paragraph{Learning in principal-agent problems}
The work that is most related to ours is the one by~\citet{zhu2022sample}, which investigates a setting very similar to ours, though from an online learning perspective (see also our Section~\ref{sec:regret}).
%
% \citet{zhu2022sample} investigate a repeated principal-agent interaction, where the principal commits to contracts based on observed outcomes.
%
\citet{zhu2022sample} provide a regret bound of the order of $\widetilde {\mathcal{O}}(T^{1 - 1/(2m+1)})$ when the principal is restricted to constraints in $[0,1]^m$, where $m$ is the number of outcomes.
Notice that such a regret bound is ``close'' to a linear dependence on $T$, even when $m$ is very small.
In contrast, in Section~\ref{sec:regret} we show how our algorithm can be exploited to achieve a regret bound of the order of $\widetilde{\mathcal{O}}(T^{4/5})$ (independent of $m$), when the number of agent's actions $n$ is constant.
%
% which is close to be linear even for small numbers of outcomes $m$. In contrast, we show that we can achieve a regret bound of $\mathcal{O}(T^{4/5})$ by exploiting a small agent's action space. 
%
Another work that is closely related to ours is the one of~\citet{ho2015adaptive}, who focus on designing a no-regret algorithm for a particular repeated principal-agent problem.
However, their approach relies heavily relies on stringent assumptions such as the \emph{first-order stochastic dominance} condition.
%
%on the well-known FOSD (First-Order Stochastic Dominance) assumption, which limits the generality of the setting.  
\bac{Finally, \cite{cohen2022learning} study a repeated principal-agent iteraction considering a \emph{risk-averse} agent. They present a no-regret algorithm that relies on the \emph{first-order stochastic dominance} condition too. }

\paragraph{Learning in Stackelberg games}
The learning problem faced in this paper is closely related to the problem of learning an optimal strategy to commit to in Stackelberg games, where the leader repeatedly interacts with follower by observing the follower's best-response action at each iteration.
\citet{letchford2009learning} propose an algorithm for the problem requiring the leader to randomly sample a set of available strategies in order to determine agent's best-response regions.
However, the performances of such an algorithm depend on the volume of the smallest best-response region.
\citet{peng2019optimal} build upon the work by~\citet{letchford2009learning}, and they propose an algorithm whose performances are more robust being independent of the volume of the smallest best-response region.
The algorithm proposed in this paper borrows some ideas from that of~\citet{peng2019optimal}.
However, it requires considerable additional machinery to circumvent the challenge posed by the fact that the principal does \emph{not} observe agent's best-response actions, but only outcomes randomly sampled according to them.
%
%
% Our setting is closely related to repeated Stackelberg games, where a leader commits to strategies while observing the actions taken by a follower. In the context of learning the optimal leader's commitment, \cite{letchford2009learning} propose an algorithm that requires the principal to randomly sample a set of strategies in order to determine the agent's best-response regions. However, their algorithm's performance dependens on the volume of the smallest feasible region of the follower's action. In contrast,~\cite{Peng2019} introduce an algorithm that is independent of the volume of the smallest best-response region, offering more robust performance. We also notice that the algorithm we propose in the following can be seen as a generalization of the one developed by \cite{peng2019optimal}. However, our setting poses an additional challenge as we do not observe the action played by the agent, and thus, we design a suitably defined algorithms to overcame this issue.
%
%
Other related works in the Stackelberg setting are~\citep{bai2021sample}, which proposes a model in where both the leader and the follower learn through repeated interaction, and~\citep{lauffer2022noregret}, which considers a scenario where the follower’s utility is unknown to the leader, but it can be linearly parameterized.
%
% They design a no-regret learning algorithm achieving a regret bound which is sublinear in the number of time steps, compared to the best policy in hindsight.
%
% In a more recent work~\cite{bai2021sample} propose a different setting where both the principal and the follower learn an equilibrium through repeated interactions. Finally, \cite{lauffer2022noregret} consider a setting in which the follower’s utility is unknown to the leader but it can be linearly parameterized. They design a no-regret learning algorithm achieving a regret bound which is sublinear in the number of time steps, compared to the best policy in hindsight. A remarkable example of repetaded security games is represented by repeated Stackelberg security games (\cite{balcan2009protecting},\cite{tambe2011security}), in which a defender (leader) strategically allocates its limited resources to protect targets against potential attackers (followers).
